# Supplementary material for: Distinct contiguous versus separated triplet-pair multiexcitons in an intramolecular singlet fission chromophore
Source: arXiv:2310.17818 source file (2023-10-26)
Supplement: Supplementary file 1 [file PTP_Mazumdar-Supplementary.pdf]

# Distinct contiguous versus separated triplet-pair multiexcitons in an intramolecular singlet fission chromophore

Rafi Chesler,[1] Pritam Bhattacharyya,[2] A. Shukla,[3] and S. Mazumdar[1]

[1]*Department of Physics, University of Arizona Tucson, AZ 85721, USA*
[2]*Institute for Theoretical Solid State Physics, Leibniz IFW Dresden, Helmholtzstraße 20, 01069 Dresden, Germany*
[3]*Department of Physics, Indian Institute of Technology Bombay, Powai, Mumbai 400076, India*

## S.1. MOLECULAR EXCITON BASIS AND ACTIVE SPACE

### S.1.1. Molecular exciton basis.

Our goal is to obtain physical, pictorial descriptions of eigenstates. This requires distinguishing between ne-nh (n = 1-4) excitations localized within monomer segments and those that are delocalized across monomers. We rewrite the PPP Hamiltonian in the main text as $H = H_{intra} + H_{inter}$ where $H_{intra} = \Sigma_\mu H^{\mu}_{intra}$ is the sum of PPP Hamiltonians describing individual molecular units $\mu$ (where $\mu$ corresponds to the two pentacene monomers and the phenylene linker) and $H_{inter} = \frac{1}{2}\Sigma\mu, \nu H^{\mu,\nu}_{inter}$ includes $t_{ij}$ and $V_{ij}$ between C atoms $i$ and $j$ belonging to different units. The calculations are now done in multiple stages. First, $H^{\mu}_{intra}$ are solved at the HF level to give MOs localized on individual units. The many-electron configurations that form the CI matrix are then constructed by repeated applications of $H_{intra} + H_{inter}$ on the most likely configurations that constitute a targeted excited state. These are 1e-1h to 4e-4h excitations from the HF ground state that can be *neutral* (number of $\pi$-electrons same as number of C atoms within each unit) and *ionic* (units positively and negatively charged).

### S.1.2. Multiple Reference CI.

The MRSDCI procedure incorporates the most dominant ne-nh excited configurations (n=1-4) that describe each targeted state. The calculation for each eigenstate is done iteratively, with each iteration consisting of two stages. In the first stage we perform a double-CI calculation on a basis space of $N_{ref}$ 1e-1h and 2e-2h configurations that best describe the targeted eigenstate. In the second stage we apply the Hamiltonian ($H_{intra} + H_{inter}$) on the $N_{ref}$ reference configurations. This generates 3e-3h and 4e-4h configurations, of which we retain the most dominant ones to give the larger Hamiltonian matrix of dimension $N_{total}$. The larger Hamiltonian matrix usually also contains new 1e-1h and 2e-2h excited configurations that were not among the original $N_{ref}$ reference configurations, but that are coupled to the 3e-3h and 4e-4h configurations reached from them. The procedure is repeated with updated $N_{ref}$ configurations to reach a new larger Hamiltonian with updated $N_{total}$, until the convergence criterion is reached. $N_{ref}$ and $N_{total}$ usually are several times $10^2$ and $10^6$, respectively.

### S.1.3. Active Space.

The MRSDCI calculations are over an active space of MOs about the chemical potential that is smaller than the complete set. The lowest few bonding MOs are frozen (i.e., excitations from these lowest MOs are not included in the CI calculations) and the highest MOs related to these by charge-conjugation symmetry are excluded from the active space. As of now, we have performed MRSDCI calculations over active spaces of 22 - 26 MOs, 11 - 13 bonding and 11 - 13 antibonding. A. Shukla has very recently been successful in performing MRSDCI calculations for 64-atom graphene quantum dots while retaining an active space of 46 MOs. These are absolutely the largest active spaces over which calculations of $^1|TT\rangle$ have ever been done.

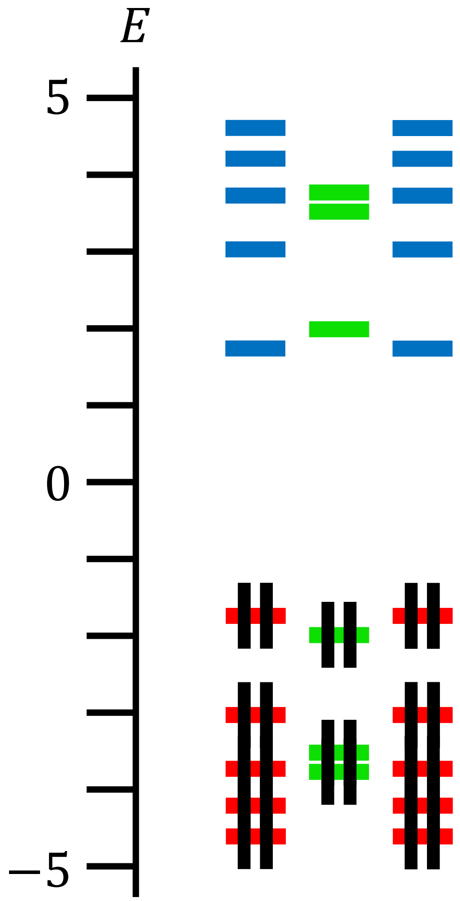


FIG. S1: Hartree-Fock (HF) energy level distribution for **P-T-P** displaying the active space of 26 MOs with pentacene bonding MOs displayed in red, pentacene antibonding MOs in blue and tetracene MOs in green. Vertical black lines denote electron occupancy, with all bonding (antibonding) MOs full (empty) in the HF ground state. Vertical overlap of occupancies is due to the energetic proximity of the MOs.

## S.2. CHARGE TRANSFER EIGENSTATES THAT PARTICIPATE IN THE GROUND STATE ABSORPTION

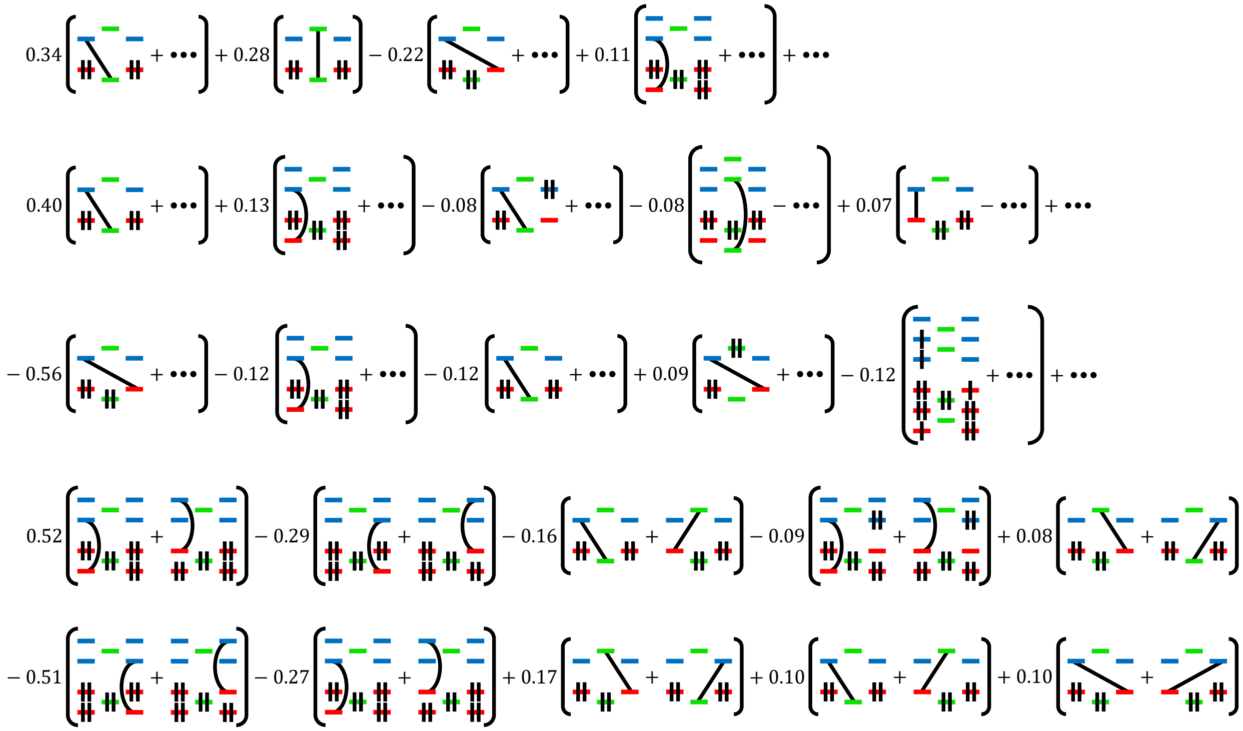


FIG. S2: Normalized CT wavefunctions for anti-**P-T-P** in the molecular exciton-basis representation that contribute to CT absorption in Fig. 1 of the text. Bonding (Antibonding) molecular orbitals (MOs) not shown in any configuration are completely filled (empty). Ellipses within parentheses correspond to additional terms related by mirror-plane and charge-conjugation symmetries. Ellipses outside parentheses indicate configurations with smaller coefficients not shown. Even in the last two eigenstates there are many such terms.

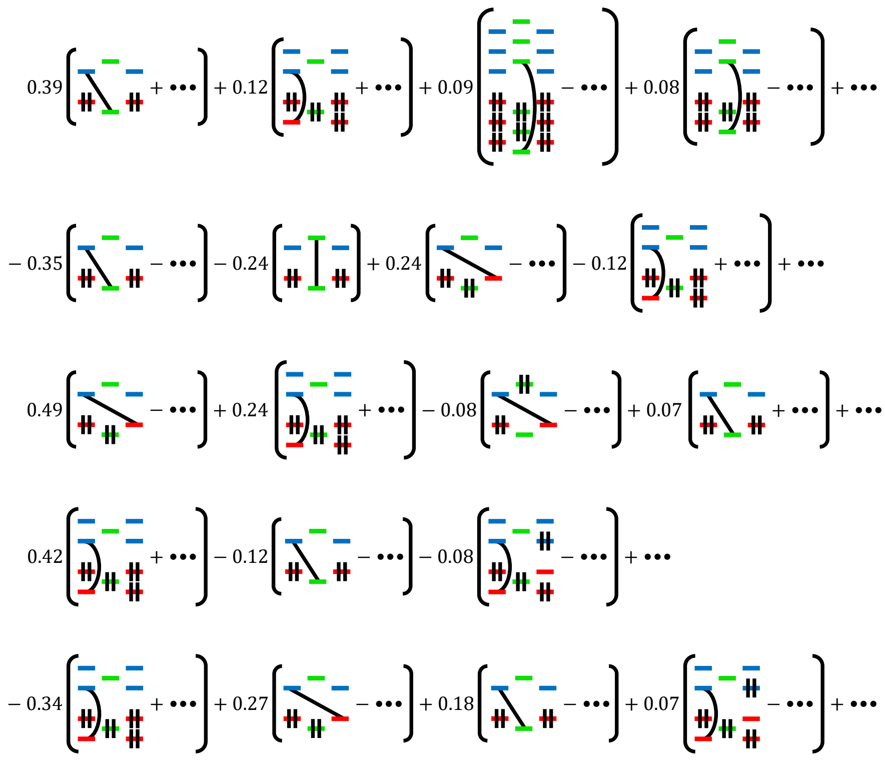

FIG. S3: Normalized CT wavefunctions for syn-**P-T-P** in the molecular exciton-basis representation that contribute to CT absorption in Fig. 1 of the text. Bonding (Antibonding) molecular orbitals (MOs) not shown in any configuration are completely filled (empty). Ellipses within parentheses correspond to additional terms related by mirror-plane and charge-conjugation symmetries. Ellipses outside parentheses indicate configurations with smaller coefficients not shown.

TABLE I: Calculated energies (in $eV$), transition dipole couplings with the ground state, and wavefunction characteristics. $\mu$ is the transition dipole coupling with the ground state (Å, electronic charge e = 1). $CT_{CC}$,$CT_{C\beta}$, and $LE_{\beta}$ are normalized coefficients of configurations displaying chromophore to chromophore CT, chromophore to bridge CT, and localized excitation on the bridge, respectively. The strongly dipole-coupled states in the charge transfer region of the absorption spectrum are dominated by contribution from configurations displaying terminal chromophore to bridge charge transfer ($CT_{C\beta}$), in contrast to the chromophore to chromophore ($CT_{CC}$) charge transfer dominated by the strongly dipole-relevant states for the molecules in S1.

| connectivity | $E$ | $\mu$ | $CT_{CC}$ | $CT_{C\beta}$ | $LE_{\beta}$ |
|---|---|---|---|---|---|
| | 3.06 | 1.49 | 0.22 | 0.34 | 0.28 |
| | 3.07 | 0.02 | 0 | 0.40 | 0.08 |
| anti | 3.29 | 0.48 | 0.56 | 0.12 | 0.06 |
| | 3.39 | 0.12 | 0.03 | 0.16 | 0.02 |
| | 3.39 | 0.39 | 0.10 | 0.17 | 0.05 |
| | 3.03 | 1.55 | 0 | 0.39 | 0.09 |
| | 3.08 | 0.47 | 0.24 | 0.35 | 0.24 |
| syn | 3.27 | 0.15 | 0.49 | 0.07 | 0.04 |
| | 3.35 | 0.34 | 0 | 0.12 | 0.03 |
| | 3.38 | 0.14 | .027 | 0.18 | 0.06 |

## S.3. CHARGE TRANSFER STATES IN THE EXCITED STATE ABSORPTION

TABLE II: Calculated energies (in $eV$), transition dipole couplings with the optical singlet state, and wavefunction characteristics. $\mu$ is the transition dipole coupling with the optical singlet state $S_1$. As in the ground state absorption, relevant states display stronger chromophore to bridge ($CT_{C\beta}$) charge transfer than chromophore to chromophore ($CT_{CC}$) charge transfer. The complete WF for the state in syn-**P-T-P** at 3.20 eV is dominated by intramonomer HOMO-1 to LUMO/HOMO to LUMO+1 excitation, not charge transfer.

| connectivity | $E$ | $\mu$ | $CT_{CC}$ | $CT_{C\beta}$ | $LE_{\beta}$ |
|---|---|---|---|---|---|
| anti | 3.04 | 1.83 | 0.16 | 0.34 | 0.07 |
| | 3.05 | 1.71 | 0 | 0.35 | 0.13 |
| | 3.22 | 1.16 | 0.03 | 0.20 | 0.10 |
| | 3.22 | 1.85 | 0.11 | 0.19 | 0.06 |
| syn | 3.01 | 1.81 | 0.14 | 0.34 | 0.12 |
| | 3.20 | 2.29 | 0.24 | 0.08 | 0.06 |
| | 3.29 | 0.66 | 0.50 | 0.07 | 0.03 |

## S.4. NORMALIZED OVERALL SPIN-SINGLET TRIPLET-TRIPLET WAVEFUNCTIONS OF SYN-P-T-P

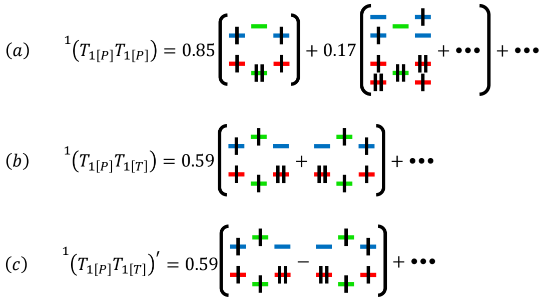


FIG. S4: Normalized wavefunctions of (a) $^1[T_{[1P]}T_{[1P]}]$, (b) and (c) $^1[T_{[1P]}T_{[1T]}]$ states in *syn*-**P-T-P**. Intramonomer excitations are spin triplet, with the overall spin zero. Observe that the configurations present are identical to those for *anti*-**P-T-P** with only the coefficients for the $^1[T_{[1P]}T_{[1T]}]$ states differing between the two sets of wavefunctions.

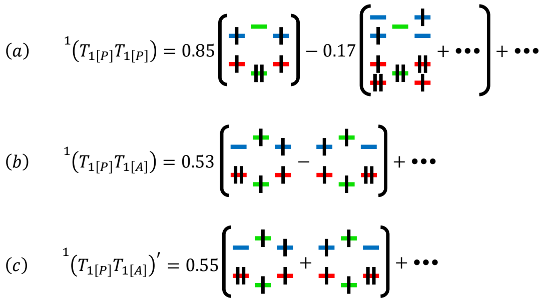


FIG. S5: Normalized wavefunctions of (a) $^1[T_{[1P]}T_{[1P]}]$, (b) and (c) $^1[T_{[1P]}T_{[1A]}]$ states in *anti*-**P-A-P**. Intramonomer excitations are spin triplet, with the overall spin zero. Observe that the configurations present are identical to those for **P-T-P** with only slight differences in the coefficients. However, the $^1[T_{[1P]}T_{[1A]}]$ states in **P-A-P** have energy 2.92 $eV$, significantly above our calculated value of 2.31 $eV$ for the optical singlet energy in **P-A-P**, thus rendering the nearest-neighbor triplet-triplet state in this molecule energetically inaccessible.

[S1] K. R. Parenti, R. Chesler, G. He, P. Bhattacharyya, B. Xiao, H. Huang, D. Malinowski, J. Zhang, X. Yin, A. Shukla, S. Mazumdar, M. Y. Sfeir, and L. M. Campos. Quantum interference effects elucidate triplet-pair formation dynamics in intramolecular singlet-fission molecules. *Nat. Chem.*, 15:339–346, 2022.
